# Supplementary material for: X-VARS: Introducing Explainability in Football Refereeing with Multi-Modal Large Language Model
Source: arXiv:2404.06332 source file (2024-04-07)
Supplement: Supplementary file 1 [file supp_qualitative_results.tex]

\begin{figure}
  \centering
  \includegraphics[width=1\linewidth]{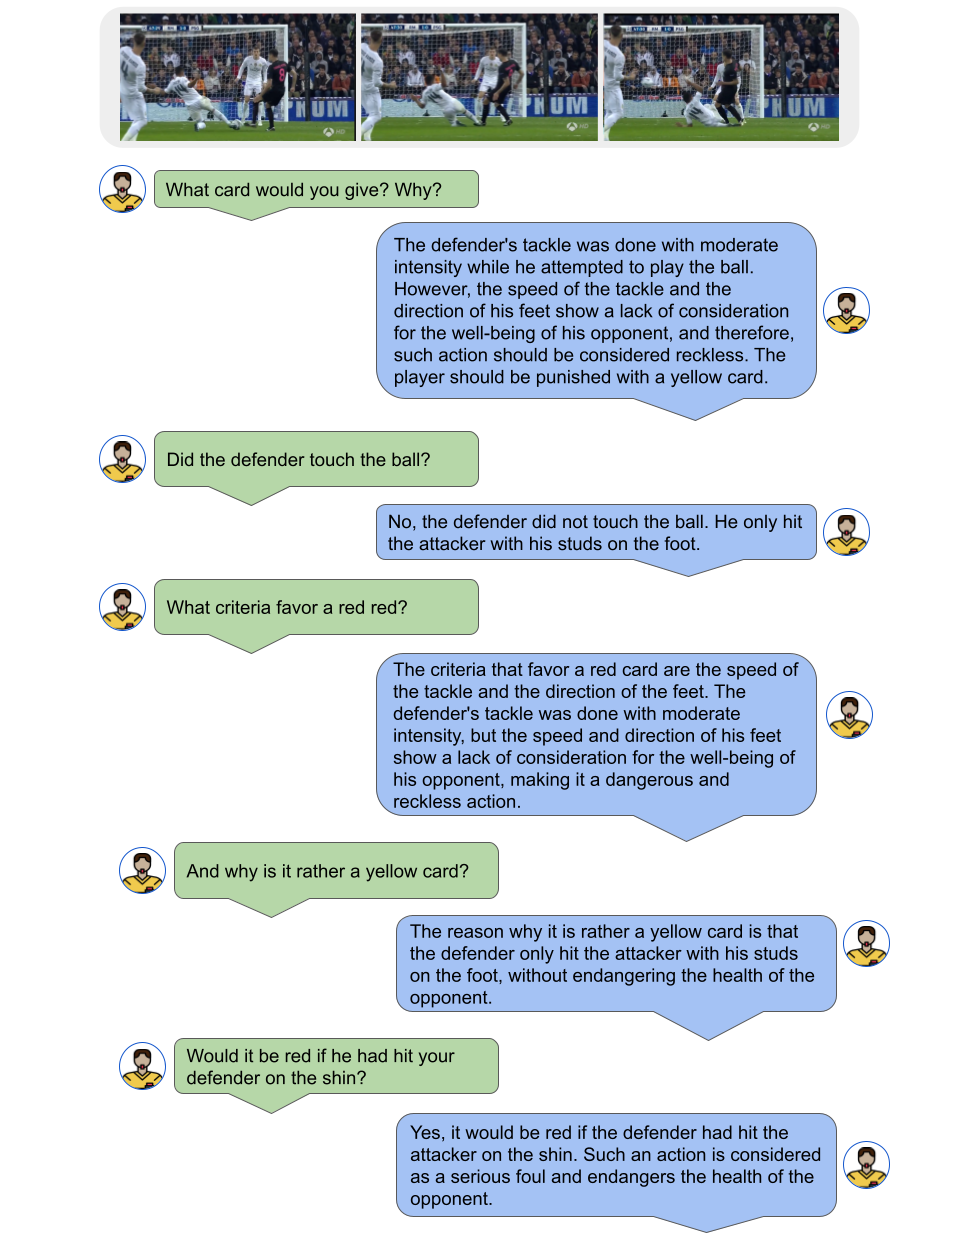}
\caption{
\textbf{Qualitiative results.} 
}
\label{fig:supp_qual_tackling}
\end{figure}
